# Supplementary material for: Giant Optomechanical Coupling in the Charge Density Wave State of Tantalum Disulfide
Source: arXiv:2105.08874 source file (2021-05-31)
Supplement: Supplementary file 1 [file SI.pdf]

# Giant Optomechanical Coupling in the Charge Density Wave State of Tantalum Disulfide

Anubhab Haldar*
*Department of Electrical and Computer Engineering,*
*Boston University, Boston, Massachusetts 02215, United States*

Cristian L. Cortes† and Stephen K. Gray‡
*Center for Nanoscale Materials, Argonne National Laboratory, Argonne, IL 60439, USA*

Sahar Sharifzadeh§
*Division of Materials Science and Engineering, Boston University, Boston, MA 02215, USA and*
*Department of Electrical and Computer Engineering, Boston University, Boston, MA 02215, USA*

Pierre Darancet¶
*Center for Nanoscale Materials, Argonne National Laboratory, Argonne, IL 60439, USA and*
*Northwestern Argonne Institute of Science and Engineering, Evanston, IL 60208, USA*

## COMPUTATIONAL DETAILS

### Density Functional Theory Calculations

The GPAW software package [1, 2] was used both for ground state DFT and optical response calculations. DFT within the generalized gradient approximation of Perdew, Burke, and Ernzerhof (PBE) [3]. We include an effective Hubbard U value of 2.27 eV calculated from first principles [4], using the procedure described in [5]. The Hubbard U value was applied inside the PAW spheres and was not normalized. We note that the application of U onto the subspace of correlated orbitals can be dependent on the precise atomic orbital projectors [6, 7] and thus, our implementation slightly differs from Ref. [4]. We utilized a planewave basis with projector augmented wave potentials to describe the core and nuclei of atoms with 5 (6) electrons considered valence for Ta (S).

The atomic and crystal structure of the high symmetry (HS) unit cell and broken symmetry (CCDW) supercell were optimized using a starting geometry from [4] until forces were less than $10^{-4}$ eV/Å. A planewave cutoff of 650 eV and a Monkhorst-Pack [8] k-point grid of $14 \times 14 \times 12$ (HS) and $4 \times 4 \times 12$ (CCDW) were used. The occupation smearing was of type Methfessel-Paxton [9] order 0 and magnitude 0.05 eV.The SCF accuracy was set to ensure convergence of the of the wavefunction residuals to below $4 \times 10^{-8}$ and the density residuals to below $10^{-4}$.

### Nudge Elastic Band Calculations

To find the minimum energy path (MEP) between two CCDW phases of $TaS_2$ (as denoted by cyan and purple arrows in Figure 1a of the manuscript), we performed nudged elastic band calculations. The NEB formulation in Ref. [10] as implemented in ASE [11] was used, and the spring constant was set to 2 eV/$\text{Å}^2$ . The initial path was created using the Image-Dependent Pair Potential (IDPP) formalism [12]. Both inter-atomic and NEB spring forces were optimized to 1 meV/Å. To aid convergence of the NEB, the first-order saddle point between the two CDW states was found using the Sella code [13], which iteratively calculates largest magnitude negative-eigenvalued eigenvector of the Hessian to converge to the saddle point. The initial guess for the saddle point image was obtained using the IDPP formalism. All forces on atoms at the saddle point were optimized to 0.1 meV/Å. This saddle point was used to create two NEB chains: one from the initial CDW to the saddle point, the other from the saddle point to the final CDW. Both chains were optimized until the magnitude of forces on all atoms were below 1 meV/Å.

### Time-dependent Density Functional Theory Calculations

The imaginary component of the dielectric function at each atomic position was calculated within the random phase approximation (RPA) [14, 15] for a series of configurations interpolated smoothly from the high-symmetry cell

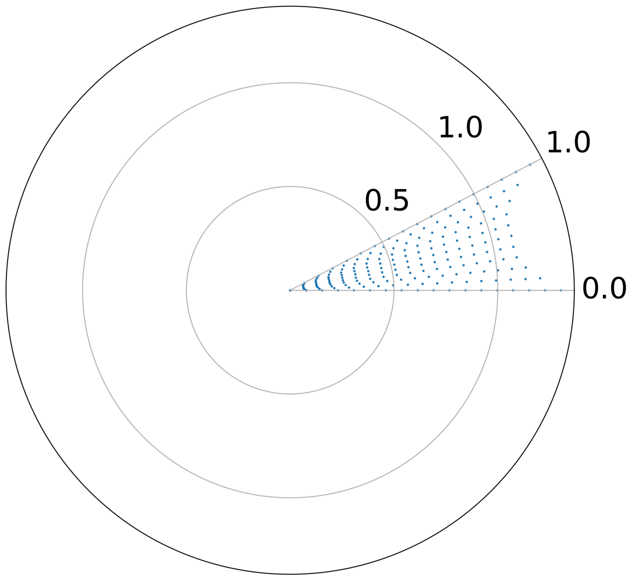


FIG. 1: The blue points correspond to configurations for which total energies and dielectric functions have been calculated. The angular direction labels correspond to fractions of $\frac{2\pi}{13}$, while the radial directions correspond to the $\ell_2$ norm of the atomic displacements.

to the two CDW configurations. Self-consistent calculations for the charge density used a 250 eV planewave cutoff, a $4 \times 4 \times 12$ kpoint grid, with a Fermi-Dirac occupation smearing of 0.05 eV. The self-consistent field was optimized until the wavefunction residual was below $1 \times 10^{-5}$ and the density residual was below $10^{-4}$. The starting orbitals and energies for the RPA were calculated via non-self-consistent DFT on 196 bands and converged until the residual was below $10^{-4}$, with a $8 \times 8 \times 12$ k-point grid to ensure a smooth dielectric function. The frequency-dependence of the dielectric function was calculated on a nonlinear frequency grid, with initial energy spacing 0.02 eV smoothly going to 0.04 eV at frequency of 10 eV. Local field effects were described with a 35 eV cutoff in the dielectric matrix. A Gaussian broadening of 0.1 eV was applied to smoothen the dielectric function. A Drude damping value $\gamma = 0.01$ eV was used in the calculation of the intraband transitions.

## CONSTRUCTING INTERPOLANTS OF THE TOTAL ENERGY AND DIELECTRIC FUNCTION

A Clough-Tocher [16, 17] interpolator as implemented in SciPy [18] was created using periodically repeating images of the total energies and dielectric functions. The Clough-Tocher interpolator is a $C^1$-smooth interpolator that can be created on an irregular grid. Our grid, shown in figure 1 contains 17 radial points at each angle for finite $r$, and 11 angular points for every value of $r > 0$. An additional point exists at $r = 0$ corresponding to the high symmetry cell.

In our reduced order model, the ‘radial’ direction (yellow arrow in Figure 1a of the manuscript) corresponds to the atomic positions moving from the high-symmetry phase to one of the 13 equivalent CCDW phases, with a given Ta atom as center. The ’angular’ direction (orange arrow in Figure 1a of the manuscript) corresponds to the atomic positions moving from a CCDW with a particular Ta atom as the center of the distortion to its nearest neighbour (NN) Ta atom as the center of distortion. The angular direction has 13-fold symmetry due to 13 possible Ta atoms which can equivalently act as a center of distortion. We calculated the potential energy surface, as well as optical properties along only a $\frac{2\pi}{13}$ slice, repeating it to the full angular extent of $2\pi$.The interpolator is used to densely sample a *uniform* grid of points in the $r - \theta$ coordinates. This dense rectangular sampled grid is subsequently used to make a SciPy RectBivariateSpline object, with quintic interpolation. This further allows analytical evaluation of derivatives without the use of finite differences, which conserves energy to high precision ($\sim 1 \times 10^{-8}$ eV) for calculation of forces. The RectBivarateSpline objects, constructed using quintic interpolation, are then used for simulations of dynamics of the configuration point in the reduced-order phase space.

## DERIVATION OF CLASSICAL EQUATIONS OF MOTION

Our framework starts from linear response theory where the interaction between light and matter is given by the Hamiltonian:

$$H_{int} = -\mathbf{P} \cdot \mathbf{E} \tag{1}$$

where $\mathbf{P}$ is a polarization vector and $\mathbf{E}$ is the electric field. It is possible show that this Hamiltonian can have contributions from the permanent dipole moment $\mathbf{d}$ as well as contributions from the polarizability $\alpha$ due to the following linear expansion:

$$\mathbf{P} = \mathbf{d} + \alpha\mathbf{E}. \tag{2}$$

IR active contributions arise from expanding the dipole moment as:

$$\mathbf{d}(\mathbf{R}) = \mathbf{d}(\mathbf{R}_o) + \frac{\partial d}{\partial R}\mathbf{R} + \frac{\partial^2 d}{\partial R^2}\mathbf{R}^2 + \cdots \tag{3}$$

Raman active contributions arise from expanding the polarizability as:

$$\alpha(\mathbf{R}) = \alpha(\mathbf{R}_o) + \frac{\partial \alpha}{\partial R}\mathbf{R} + \frac{\partial^2 \alpha}{\partial R^2}\mathbf{R}^2 + \cdots \tag{4}$$

Time-dependent DFT calculations have shown that the electronic polarizability of $TaS_2$ depends explicitly on the atomic coordinates $\mathbf{R}$. In the following, we will only consider Raman-active contributions.

### Hamiltonian model

Assuming a single vector coordinate for simplicity, the total Hamiltonian in the presence of a driving field $\mathbf{E}$ and subject to the potential, $U(\mathbf{R})$, may be written as:

$$H = \tfrac{1}{2}\mathbf{p}^2 + U(\mathbf{R}) - \mathbf{P} \cdot \mathbf{E}. \tag{5}$$

Using the results from the previous section, it is possible to show that this Hamiltonian gives rise to parametric and nonlinear effects. Assuming a Cartesian coordinate system, we derive Hamilton's equations of motion:

$$\dot{\mathbf{p}} = -\frac{\partial}{\partial R}U(\mathbf{R}) + \frac{\partial}{\partial R}(\mathbf{P} \cdot \mathbf{E}) \;\text{ and }\; \dot{\mathbf{R}} = \mathbf{p} \tag{6}$$

allowing us to find the equation of motion for the coordinate vector $\mathbf{R}$:

$$\ddot{\mathbf{R}} = -\frac{\partial}{\partial R}U(\mathbf{R}) + \mathbf{E}\frac{\partial \alpha(\mathbf{R})}{\partial R}\mathbf{E}. \tag{7}$$

This equation defines the fundamental equation of motion for a single coordinate vector $\mathbf{R}$ in the presence of a driving field. Note that it is possible to add a phenomenological damping term $\kappa\dot{\mathbf{R}}$ to the left hand side of the equation, thereby accounting for realistic damping. The derivation of the equations of motion for the Higgs and Goldstone modes follows in a straightforward way from the derivation presented above. We provide the final expressions written in equations 20 and 21.

### Equations of motion in the Higgs and Goldstone Coordinates

We start by writing down expressions for forces in the radial and angular directions, within the (polar) coordinates of the symmetry-breaking potential:

$$F_r = ma_r \tag{8}$$

$$F_\theta = ma_\theta \tag{9}$$

Where $a_r$ and $a_\theta$ are the radial and angular accelerations respectively.

In these coordinates, the acceleration terms are given by the equations:

$$a_r = \ddot{r} - r\dot{\theta}^2 \tag{10}$$

$$a_\theta = 2\dot{r}\dot{\theta} + r\ddot{\theta} \tag{11}$$

The acceleration terms can alternatively be described in terms of the gradient of the potential energy surface associated with application of each mode:

$$a_r = -\frac{\boldsymbol{\nabla}_r U}{m} = -\frac{1}{m}\frac{\partial U}{\partial r} \tag{12}$$

$$a_\theta = -\frac{\boldsymbol{\nabla}_\theta U}{m} = -\frac{1}{mr}\frac{\partial U}{\partial \theta}, \tag{13}$$

where $m$ is the mass of the phonon mode. Including the external force that drives the phase transition, and a dissipation to model realistic systems, gives:

$$a_r = \frac{1}{m}\left(-\frac{\partial U}{\partial r} - \kappa_r \dot{r} - \frac{\partial \alpha}{\partial r}E^2\right) \tag{14}$$

$$a_\theta = \frac{1}{m}\left(-\frac{1}{r}\frac{\partial U}{\partial \theta} - \kappa_\theta r, \dot{\theta} - \frac{1}{r}\frac{\partial \alpha}{\partial \theta}E^2\right) \tag{15}$$

, where $\kappa_r$ and $\kappa_\theta$ are the radial and angular direction damping constants, respectively. Rearranging Equations 14-15 gives:

$$\ddot{r} - r\dot{\theta}^2 = \frac{1}{m}\left(-\frac{\partial U}{\partial r} - \kappa_r \dot{r} - \frac{\partial \alpha}{\partial r}E^2\right) \tag{16}$$

$$\ddot{r} = -\frac{1}{m}\left(\frac{\partial U}{\partial r} + \kappa_r \dot{r} + \frac{\partial \alpha}{\partial r}E^2\right) + r\dot{\theta}^2 \tag{17}$$

and

$$2\dot{r}\dot{\theta} + r\ddot{\theta} = \frac{1}{m}\left(-\frac{1}{r}\frac{\partial U}{\partial \theta} - \kappa_\theta r\dot{\theta} - \frac{1}{r}\frac{\partial \alpha}{\partial \theta}E^2\right) \tag{18}$$

$$\ddot{\theta} = -\frac{1}{mr}\left(\frac{1}{r}\frac{\partial U}{\partial \theta} + \kappa_\theta r\dot{\theta} + \frac{1}{r}\frac{\partial \alpha}{\partial \theta}E^2\right) - \frac{2\dot{r}\dot{\theta}}{r} \tag{19}$$

Equations 17 and 19 are then solved using an ordinary differential equation (ODE) integrator to obtain the classical dynamics trajectories.

$$m\ddot{\mathbf{r}} = \frac{\partial U}{\partial \mathbf{r}} + \kappa\dot{\mathbf{r}} + R\left[\mathbf{r}\right]\mathbf{E}^2 \tag{20}$$

$$m\ddot{\boldsymbol{\Theta}} = \frac{\partial U}{\partial \boldsymbol{\Theta}} + \kappa\dot{\boldsymbol{\Theta}} + R\left[\boldsymbol{\Theta}\right]\mathbf{E}^2 \tag{21}$$

## CLASSICAL EQUATIONS OF MOTION FOR THE DYNAMIC EVOLUTION OF ATOMS

### Integrator

Classical dynamics of points in configuration space (corresponding to particular atomic configurations) were performed using SciPy's solve_ivp method. The DOP853 integrator was used, and the solution was interpolated to a dense time grid using a seventh-order interpolating polynomial. Both relative and absolute tolerances of integration are set to $10^{-13}$ in the integration and the trajectory is integrated using the classical equations of motion as detailed below.

| Reference Number | Measurement | Pulse parameters | Response | Comments |
|---|---|---|---|---|
| [20] | TR-PES | 1.5 eV / 50 fs | 2.45 THz and 2.51 THz. Decay time 9.5 ps. | High intensity pulse (0.1 e / unit cell). |
| [21] | Femtosecond electron diffraction | 3.2 eV / 150 fs | 2.3 THz coherent amplitude mode and phonon mode at 2.1 THz. | Measured using differential reflectivity at 1.55 eV (800 nm). |
| [22] | TR reflectivity changes | 1.3 $\mu$m (950 meV) / Not found | 2.4 THz coherent CDW mode. | Reflectivty changes, best seen at 0.62 eV probe energies. |
| [23] | TR-ARPES | 790 nm (1.57 eV) / 30 fs FWHM | 412+-5 fs time period of intensity modulation near the $\overline{M}$ point. | EXTRACTED: 2.43 THz / 0.46 THz damping from model fit line (black in figure 4, fit to yellow dots). |
| [24] | MeV transmission electron diffraction after optical pulse | 800 nm (1.55 eV) / 80 fs | 2.35 THz intensity modulation of Bragg peaks in large-domain samples. 2.25 THz in small-domain samples. | EXTRACTED: 2.37 THz / 0.25 THz damping from model fit line (blue in figure 3b). |
| [25] | TR-PES | 1.55 eV / 50 fs | 2.5 THz | EXTRACTED: 2.3 and 2.4 THz from yellow curve in figure 4 fit to 2 decaying sines. |
| [26] | TR-Reflectivity | 800 nm (1.55 eV) / 50 fs | 2.45 THz | Data extracted from figure 1 a. |
| [27] | Raman | 2.41 eV CW | 2.5 THz | - |

TABLE I: Experimental measurements of the optical excitation of the 2.4 THz phonon mode in 1T-$TaS_2$. This phonon mode couples very strongly to changes in the dielectric function along the CDW amplitude coordinate, resulting in a large coupling to external electromagnetic fields.

## EXPERIMENTAL PARAMETERS FROM PREVIOUS WORKS

Data labeled EXTRACTED has been extracted from figures cited references using WebPlotDigitizer [19].

## DIELECTRIC FUNCTION

* ahaldar@bu.edu
† ccortes@anl.gov
‡ gray@anl.gov
§ ssharifz@bu.edu
¶ pdarancet@anl.gov
[1] J. J. Mortensen, L. B. Hansen, and K. W. Jacobsen, Real-space grid implementation of the projector augmented wave method, Physical Review B **71**, 035109 (2005).
[2] J. Enkovaara, C. Rostgaard, J. J. Mortensen, J. Chen, M. Dułak, L. Ferrighi, J. Gavnholt, C. Glinsvad, V. Haikola, H. A. Hansen, H. H. Kristoffersen, M. Kuisma, A. H. Larsen, L. Lehtovaara, M. Ljungberg, O. Lopez-Acevedo, P. G. Moses, J. Ojanen, T. Olsen, V. Petzold, N. A. Romero, J. Stausholm-Møller, M. Strange, G. A. Tritsaris, M. Vanin, M. Walter, B. Hammer, H. Häkkinen, G. K. H. Madsen, R. M. Nieminen, J. K. Nørskov, M. Puska, T. T. Rantala, J. Schiøtz, K. S.

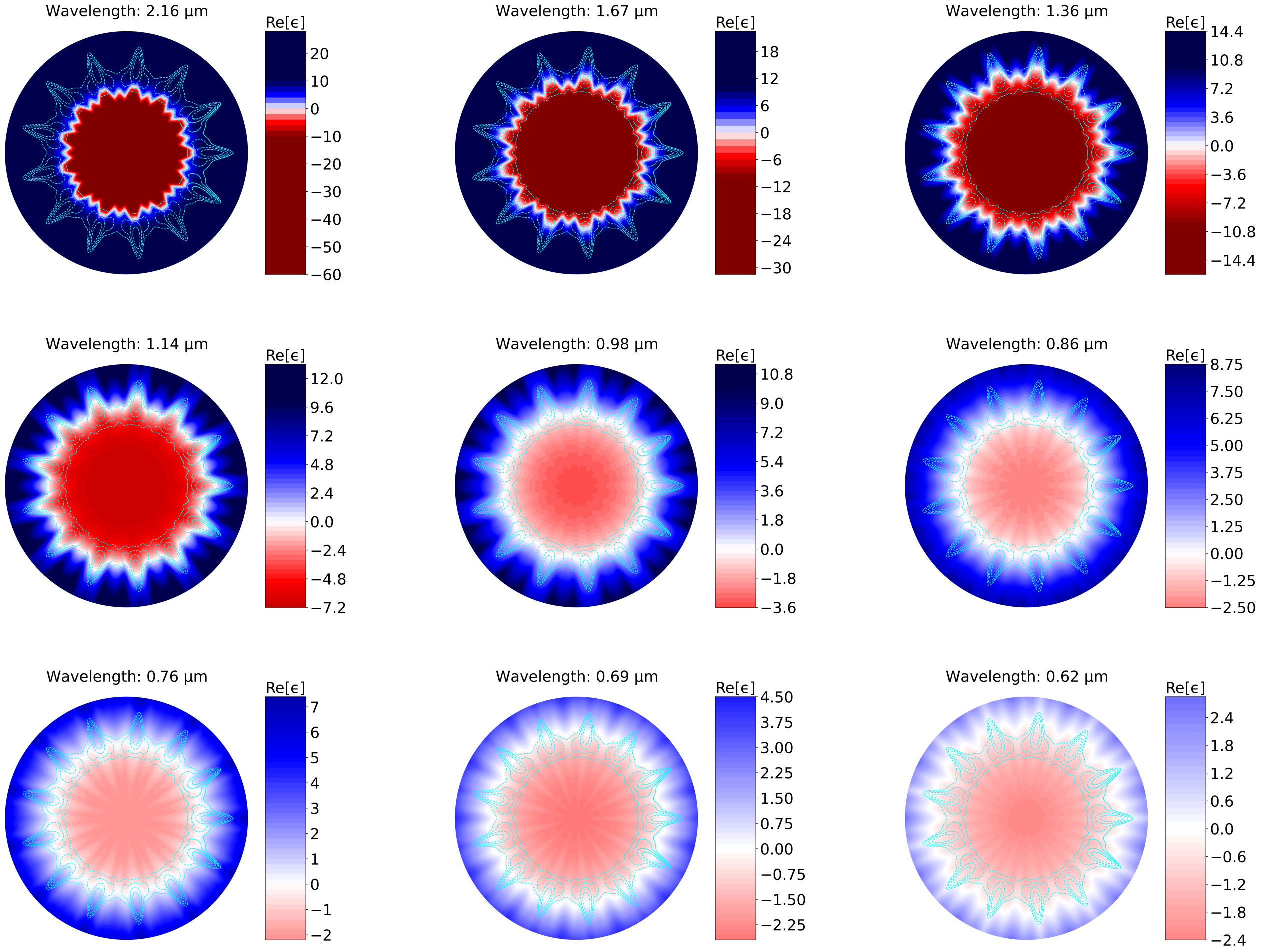


FIG. 2: Real part of the dielectric function along the CDW normal mode coordinate at different energies. For all energies, the zero of the colobar is set to white.

Thygesen, and K. W. Jacobsen, Electronic structure calculations with GPAW: A real-space implementation of the projector augmented-wave method, Journal of Physics: Condensed Matter **22**, 253202 (2010).
[3] J. P. Perdew, K. Burke, and M. Ernzerhof, Generalized gradient approximation made simple, Physical review letters **77**, 3865 (1996).
[4] P. Darancet, A. J. Millis, and C. A. Marianetti, Three-dimensional metallic and two-dimensional insulating behavior in octahedral tantalum dichalcogenides, Phys. Rev. B **90**, 045134 (2014).
[5] M. Cococcioni and S. de Gironcoli, Linear response approach to the calculation of the effective interaction parameters in the LDA + U method, Physical Review B **71**, 035105 (2005).
[6] N. E. Kirchner-Hall, W. Zhao, Y. Xiong, I. Timrov, and I. Dabo, Extensive benchmarking of dft+ u calculations for predicting band gaps, Applied Sciences **11**, 2395 (2021).
[7] M. Kick, K. Reuter, and H. Oberhofer, Intricacies of dft+ u, not only in a numeric atom centered orbital framework, Journal of chemical theory and computation **15**, 1705 (2019).
[8] H. J. Monkhorst and J. D. Pack, Special points for Brillouin-zone integrations, Physical Review B **13**, 5188 (1976).
[9] M. Methfessel and A. T. Paxton, High-precision sampling for Brillouin-zone integration in metals, Physical Review B **40**, 3616 (1989).
[10] G. Henkelman, B. P. Uberuaga, and H. Jónsson, A climbing image nudged elastic band method for finding saddle points and minimum energy paths, The Journal of Chemical Physics **113**, 9901 (2000).
[11] A. H. Larsen, J. J. Mortensen, J. Blomqvist, I. E. Castelli, R. Christensen, M. Du\lak, J. Friis, M. N. Groves, B. Hammer, C. Hargus, E. D. Hermes, P. C. Jennings, P. B. Jensen, J. Kermode, J. R. Kitchin, E. L. Kolsbjerg, J. Kubal, K. Kaasbjerg, S. Lysgaard, J. B. Maronsson, T. Maxson, T. Olsen, L. Pastewka, A. Peterson, C. Rostgaard, J. Schiøtz, O. Schütt, M. Strange, K. S. Thygesen, T. Vegge, L. Vilhelmsen, M. Walter, Z. Zeng, and K. W. Jacobsen, The atomic simulation environment—a Python library for working with atoms, J. Phys.: Condens. Matter **29**, 273002 (2017).
[12] S. Smidstrup, A. Pedersen, K. Stokbro, and H. Jónsson, Improved initial guess for minimum energy path calculations, The Journal of Chemical Physics **140**, 214106 (2014).
[13] E. D. Hermes, K. Sargsyan, H. N. Najm, and J. Zádor, Accelerated Saddle Point Refinement through Full Exploitation of Partial Hessian Diagonalization, Journal of Chemical Theory and Computation **15**, 6536 (2019).
[14] D. Pines and D. Bohm, A Collective Description of Electron Interactions: II. Collective $\mathrm{vs}$ Individual Particle Aspects of the Interactions, Physical Review **85**, 338 (1952).
[15] G. D. Mahan, *Many-Particle Physics*, 3rd ed. (Springer US, New York, 2000).
[16] P. Alfeld, A trivariate clough—tocher scheme for tetrahedral data, Computer Aided Geometric Design **1**, 169 (1984).
[17] G. Farin, Triangular Bernstein-Bézier patches, Computer Aided Geometric Design **3**, 83 (1986).
[18] P. Virtanen, R. Gommers, T. E. Oliphant, M. Haberland, T. Reddy, D. Cournapeau, E. Burovski, P. Peterson, W. Weckesser, J. Bright, S. J. van der Walt, M. Brett, J. Wilson, K. J. Millman, N. Mayorov, A. R. J. Nelson, E. Jones, R. Kern, E. Larson, C. J. Carey, İ. Polat, Y. Feng, E. W. Moore, J. VanderPlas, D. Laxalde, J. Perktold, R. Cimrman, I. Henriksen, E. A. Quintero, C. R. Harris, A. M. Archibald, A. H. Ribeiro, F. Pedregosa, P. van Mulbregt, and S. . . Contributors, SciPy 1.0–Fundamental Algorithms for Scientific Computing in Python, arXiv:1907.10121 [physics] (2019), arXiv:1907.10121 [physics].
[19] A. Rohatgi, Webplotdigitizer: Version 4.4 (2020).
[20] L. Perfetti, P. A. Loukakos, M. Lisowski, U. Bovensiepen, H. Berger, S. Biermann, P. S. Cornaglia, A. Georges, and M. Wolf, Time Evolution of the Electronic Structure of 1 T - TaS 2 through the Insulator-Metal Transition, Physical Review Letters **97**, 067402 (2006).
[21] M. Eichberger, H. Schäfer, M. Krumova, M. Beyer, J. Demsar, H. Berger, G. Moriena, G. Sciaini, and R. J. D. Miller, Snapshots of cooperative atomic motions in the optical suppression of charge density waves, Nature **468**, 799 (2010).
[22] N. Dean, J. C. Petersen, D. Fausti, R. I. Tobey, S. Kaiser, L. V. Gasparov, H. Berger, and A. Cavalleri, Polaronic Conductivity in the Photoinduced Phase of 1 T - TaS 2, Physical Review Letters **106**, 016401 (2011).
[23] S. Hellmann, T. Rohwer, M. Kalläne, K. Hanff, C. Sohrt, A. Stange, A. Carr, M. Murnane, H. Kapteyn, L. Kipp, *et al.*, Time-domain classification of charge-density-wave insulators, Nature communications **3**, 1 (2012).
[24] A. Zong, X. Shen, A. Kogar, L. Ye, C. Marks, D. Chowdhury, T. Rohwer, B. Freelon, S. Weathersby, R. Li, J. Yang, J. Checkelsky, X. Wang, and N. Gedik, Ultrafast manipulation of mirror domain walls in a charge density wave, Science Advances **4**, eaau5501 (2018).
[25] I. Avigo, P. Zhou, M. Kalläne, K. Rossnagel, U. Bovensiepen, and M. Ligges, Excitation and Relaxation Dynamics of the Photo-Perturbed Correlated Electron System 1T-TaS2, Applied Sciences **9**, 44 (2018).
[26] J. Demsar, L. Forró, H. Berger, and D. Mihailovic, Femtosecond snapshots of gap-forming charge-density-wave correlations in quasi-two-dimensional dichalcogenides 1 T - TaS 2 and 2 H - TaSe 2, Physical Review B **66**, 041101 (2002).
[27] S. Sugai, Lattice Vibrations in the Charge-Density-Wave States of Layered Transition Metal Dichalcogenides, physica status solidi (b) **129**, 13 (1985).
